# Supplementary material for: Observation of Majorization Principle for quantum algorithms via 3-D integrated photonic circuits
Source: arXiv:1608.01141 ancillary file (2016-08-03)
Supplement: Supplementary file 1 [file Supplementary_Information.pdf]

# Observation of Majorization Principle for quantum algorithms via 3-D integrated photonic circuits

## — Supplemental Material —

Fulvio Flamini,<sup>1</sup> Niko Viggianiello,<sup>1</sup> Taira Giordani,<sup>1</sup> Marco Bentivegna,<sup>1</sup> Nicolò Spagnolo,<sup>1</sup> Andrea Crespi,<sup>2,3</sup> Giacomo Corrielli,<sup>2</sup> Roberto Osellame,<sup>2,3</sup> M. A. Martin-Delgado,<sup>4</sup> and Fabio Sciarrino<sup>1,\*</sup>

<sup>1</sup>*Dipartimento di Fisica, Sapienza Università di Roma, Piazzale Aldo Moro 5, I-00185 Roma, Italy*

<sup>2</sup>*Istituto di Fotonica e Nanotecnologie, Consiglio Nazionale delle Ricerche (IFN-CNR),  
Piazza Leonardo da Vinci, 32, I-20133 Milano, Italy*

<sup>3</sup>*Dipartimento di Fisica, Politecnico di Milano, Piazza Leonardo da Vinci, 32, I-20133 Milano, Italy*

<sup>4</sup>*Departamento de Física Teórica I, Universidad Complutense, 28040 Madrid, Spain*

### Quantum-to-Classical transition

We briefly discuss the observation of the Majorization Principle while changing the degree of distinguishability between the input photons in the validation protocol. Since the quantum validation protocol is based on genuine bosonic interference, it is fundamental to investigate how partial photon distinguishability influences the correspondent Lorenz diagrams. In the experimental realization, photons undergoing the Fourier transformation are not completely identical due to unavoidable imperfections in the state preparation. Specifically, a quantum-to-classical transition is observed while varying the time delay  $\Delta\tau$  between the injected photons. The scattering probability for the output configuration  $T$ , after the evolution  $U$  and given the input  $S$ , can be calculated as [1]

$$\mathcal{P}_{ST}(\Delta\tau) = \frac{1}{2} \left( \frac{\text{per } U_{ST}}{\det U_{ST}} \right)^\dagger \begin{pmatrix} 1 + \alpha & 0 \\ 0 & 1 - \alpha \end{pmatrix} \left( \frac{\text{per } U_{ST}}{\det U_{ST}} \right)$$

being  $\alpha = \zeta e^{-\xi \Delta\tau^2}$ , where  $\zeta$  and  $\xi$  take into account differences in frequencies  $\omega_1, \omega_2$  and spectral widths  $\sigma_1, \sigma_2$  respectively. We assume that both photons have the same frequency and spectral width, so  $\zeta = 1$  and  $\xi = \frac{\sigma^2}{2}$ .  $U_{S,T}$  is a  $2 \times 2$  submatrix of  $U$ .

The indistinguishability is reached for  $\Delta\tau \rightarrow 0$ : the wave function is symmetric in accordance with the bosonic statistics, so we have only the contribution of the permanents. The contribution of the determinants increases with  $\Delta\tau$ , until the two weights become the same for  $\Delta\tau \rightarrow \infty$ : it is the classical scenario in which photons are perfectly distinguishable and the wave function does not have any specific symmetry. This formula is not relevant for input states with both photons in the same mode, since they do not interfere. Indeed, their output probability distribution does not depend to the optical delay. For two-photon interference,  $\mathcal{P}_{ST}(\Delta\tau)$  is a monotonic function of the delay [2], thus the Majorization Principle is always verified for all  $\Delta\tau$ .

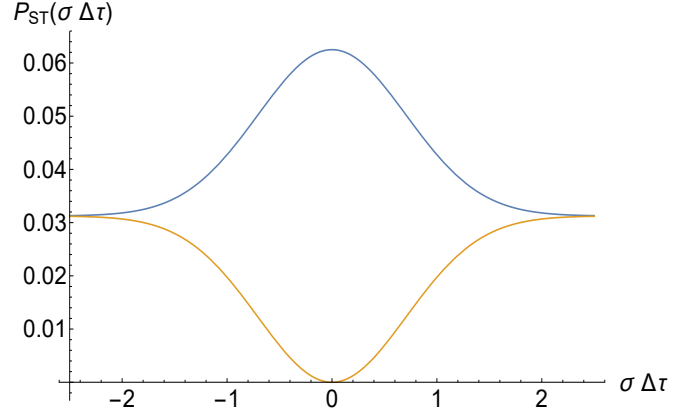

FIG. 1: Ideal monotonic quantum-to-classical transition in a Fourier interferometer for the cyclic input of the validation algorithm. The orange line refers to a suppressed output configuration, the blue one to an enhanced configuration. Dip and peak visibilities are equal to 1 and -1, respectively.

### Classes in QFT 2-photon output probabilities

Due to the internal symmetries in the QFT, it is possible to classify the states according to their Lorenz plot in a Majorization experiment. It can be shown that, for a  $2^t$ -dimensional QFT, there exist  $t + 1$  classes  $\{c\}$  collecting all 2-photon states  $(m_1, m_2)$  which satisfy

$$c_{(m_1, m_2)} + s^* = t \quad (1)$$

where  $s^*$  is the first different bit in the binary representation of the two modes  $(m_1, m_2)$ , starting the comparison from the rightmost one.

The proof can be sketched as follows. First, we know that the scattering probability  $p_{i,j}^{k,l}$ , where  $(i, j)$  and  $(k, l)$  are the input and output 2-photon states respectively, is the same within each class. For pairs of indistinguishable photons injected into an interferometer implementing a unitary transformation  $(U)_{i,j} = u_{i,j}$

$$p_{i,j}^{k,l} \propto |\text{per } c_{i,j}^{k,l}|^2 = |u_{k,i}u_{l,j} + u_{k,j}u_{l,i}|^2 \quad (2)$$

which in the case of a QFT becomes proportional to the quantity  $\left| e^{2\pi i \frac{k_i}{d}} e^{2\pi i \frac{l_j}{d}} + e^{2\pi i \frac{k_j}{d}} e^{2\pi i \frac{l_i}{d}} \right|^2$ .

From here, observing that  $|e^{i\alpha} + e^{i\beta}|^2 \propto \cos^2(\frac{\beta-\alpha}{2})$ , we directly find

$$p_{i,j}^{k,l} \propto 1 + \cos\left(\frac{2\pi}{d} (l-k)(j-i)\right) \quad (3)$$

Let us now define the quantities  $\Delta_{kl} = |k-l|$  and  $\Delta_{ij} = |i-j|$ , whence

$$p_{i,j}^{k,l} \propto 1 + \cos\left(\frac{2\pi}{d} \Delta_{kl} \Delta_{ij}\right) \quad (4)$$

Suppose that the input modes  $(i, j)$  belong to the same class  $C_{a,b}$  of the input modes  $(a, b)$ , over a set of classes whose cardinality is yet to be determined. Let us also write  $\Delta_{ij} = \Delta_{ab} + n_{i,j} 2^{c_{i,j}}$ , with  $\gcd(n_{i,j}, 2) = 1$ . We then require, for the two pairs of modes  $(i, j)$  and  $(a, b)$  to belong to the same class  $C_{a,b}$ , that  $p_{i,j}^{k,l} = p_{a,b}^{k,l}$ , i.e.

$$\begin{aligned} \cos\left(\frac{2\pi}{d} \Delta_{kl} \Delta_{ij}\right) &= \cos\left(\frac{2\pi}{d} \Delta_{kl} \Delta_{ab}\right) = \\ &= \cos\left[\frac{2\pi}{d} \Delta_{kl} (\Delta_{ab} + n_{i,j} 2^{c_{i,j}})\right] \end{aligned} \quad (5)$$

from which we have to satisfy  $\text{mod}(\Delta_{kl} n_{i,j} 2^{c_{i,j}}, d) = 0$ . By using the binary representation, we can recast the equation as

$$\text{mod}\left(n_{i,j} \sum_{s=0}^{\log_2(d)-1} \left(b_s^{(k)} - b_s^{(l)}\right) 2^{c_{i,j}+s}, d\right) = 0 \quad (6)$$

For a  $2^t$ -dimensional QFT we can then write, by recalling also that  $\gcd(n_{i,j}, 2) = 1$ ,

$$\begin{aligned} \text{mod}\left(n_{i,j} \sum_{s=0}^{t-1} \left(b_s^{(k)} - b_s^{(l)}\right) 2^{c_{i,j}+s}, 2^t\right) &= \\ = \text{mod}\left(\sum_{s=0}^{t-1} \delta_{b_s^{(k)}, b_s^{(l)}} 2^{c_{i,j}+s}, 2^t\right) &= 0 \end{aligned} \quad (7)$$

which finally determines the class  $C_{i,j} = c_{i,j}$  to which  $(i, j)$  belongs. All we require is in fact that  $c_{i,j} + s^* = t$ , where  $s^*$  is the position of first bit, starting from the right, to be different between the binary representations of the two modes  $(i, j)$ .

---

\* Electronic address: [fabio.sciarrino@uniroma1.it](mailto:fabio.sciarrino@uniroma1.it)

1. M. Tillmann, S. H. Tan, S. E. Stoeckl, B. C. Sanders, H. de Guise, R. Heilmann, S. Nolte, A. Szameit, P. Walther, Phys. Rev. X **5**, 041015 (2015).
2. Y. S. Ra, M. C. Tichy, H. T. Lim, O. Kwon, F. Mintert, A. Buchleitner, and Y. H. Kim, PNAS **110** (4) 1227 (2013).
